# Supplementary material for: Search-based Motion Planning for Quadrotors using Linear Quadratic Minimum Time Control
Source: arXiv:1709.05401 source file (2017-09-15)
Supplement: Supplementary file 1 [file Appendix.tex]

\section*{Appendix}
\section{Optimal State Trajectories}
\label{app:a}
If the constraint $x(t) \in \mathcal{X}^{free}$ in Problem \eqref{eq: problem1} is removed, the optimal state trajectory of the relaxed problem can be obtained using Pontryagin's minimum principle as suggested in \cite{mueller2015}. For simplicity, we show a derivation for $n=2$ so that the state $x(t) := \brl{p^T\;v^T}^T$ consists of position $p(t)$ and velocity $v(t) = \dot{p}(t)$, while the control input is measured by the squared norm of acceleration $u(t) = a(t) = \ddot{p}(t)$. The fully-actuated dynamics are:
\[
\dot{x} = f(x,a) = \brl{v^T\;a^T}^T.
\]
We introduce the costate $\lambda:=\brl{\lambda_v^T\;\lambda_a^T}^T$ and define the Hamiltonian:
\[
H(x,a,\lambda) = a^Ta + \lambda_v^Tv + \lambda_a^Ta
\]
The costate differential equation is:
\[
\dot{\lambda} = -\nabla_x H(x^*,a^*,\lambda) = \brl{0^T\;-\lambda_v^T}^T
\]
where $x^*$ and $a^*$ are the optimal state and input trajectories, respectively. The solution of the costate equation can be written for convenience as:
\[
\lambda(t) := \begin{bmatrix} 2b_3 \\ -2b_3t-2b_2 \end{bmatrix} 
\]
which results in:
\[
a^*(t) = \argmin_{a(t)} H(x^*(t),a(t),\lambda(t)) = b_3t + b_2
\]
and integration of $a^*$ leads to the following optimal state trajectory:
\begin{equation}\label{eq: kinematic}
x^*(t) = \begin{bmatrix}
  \frac{b_3}{6}t^3 + \frac{b_2}{2} t^2 + b_1 t + b_0\\
  \frac{b_3}{2}t^2 + b_2t + b_1
\end{bmatrix}
\end{equation}
The same procedure can be used for a derivation of a higher order $n \geq 3$. We see that a polynomial of degree $m = 2n-1$ is sufficient to represent the optimal trajectory and for specified initial and final states ($2\times(3n)$ constraints), the $3\times(2n)$ coefficients $b_0,\ldots,b_{2n-1}$ can be determined. 

%Refer to Eq.~\ref{eq: poly}, we can easily see that 
%\begin{align}
%m &= 2n-1\\
%b_k &= \frac{c_k}{k!}, \quad k = 0,\ldots,m
%\end{align}


 
